# Supplementary material for: Cash Accumulation Strategy based on Optimal Replication of Random Claims with Ordinary Integrals
Source: arXiv:1711.01756 source file (2017-11-06)
Supplement: Supplementary file 1 [file appendices.tex]

\section*{Appendices}

\begin{lstlisting}[frame=none]
clear 
% Define end of time interval
T=1;
N = 365;
dt = T/N;
%Define number of dimensions
m = 2;

W = zeros(m,N);
dW = zeros(m,N);
x= zeros(m,N); 

if m == 1
    W0 = 150;
    a = @(z) 0;
    sigma = @(z)0.5;
    start = 50;
end

if m ==2
    W0 = [200;
        400];
    a = @(z) [0;
        0];    
    sigma = @(z) 1;
    start = [20,
        20];
end

a = @(z) 0;
sigma =  @(z)0.5;
for i=1:N
    if i ==1 
        dW(:,1) = W0 .*( a(i*dt) .* dt + sigma(i*dt) .* sqrt(dt) .* randn(m,1));
        W(:,1) = W0 + dW(:,1);
    else
        dW(:,i) = W(:,i-1) .*( a(i*dt).* dt+  sigma(i*dt) .*  sqrt(dt).*randn(m,1));
        W(:,i) = W(:,i-1) + dW(:,i); 
    end
end

Gamma = @(t)1; 
ir = 0.3;
A = ir;
Q= @(x) exp(2*A*(T-x)).*Gamma(x).^(-1); 
R = @(s) quad(Q,s,T); 
M = 0;

for q = 1:N
    t = q*dt;
    r = R(t);
    M = M + r.^(-1) * dW(:,q);
    mu = R(0).^(-1)*(W0 - exp(A*T).*start) + M;
    u = Gamma(t).^(-1)*exp(A*(T-t))*mu;
    if q == 1
        x(:,1) = exp(ir*dt).*(start + u*dt);
    else
        x(:,q) = (x(:,q-1) + u*dt).*exp(ir*dt);
    end
end   
figure
if m==1
    plot( 0:dt:T, [W0,W]) 
    hold on
    plot( 0:dt:T, [start, x])
else
    plot(0:dt:T, [sum(W0), sum(W)])
    hold on
    plot( 0:dt:T, [sum(start), sum(x)])
end
hold on
xlabel('Time (years)')
ylabel('Value ($)')
legend( 'Stock Price', 'Accumulated Cash')
matlab2tikz('21.tex')

if m == 2
    figure
    plot( 0:dt:T, [W0(1),W(1,:)] )
    hold on 
    plot( 0:dt:T, [W0(2),W(2,:)], 'black')
    xlabel('Time (years)')
    ylabel('Dollars ($)')
    legend('Stock Price 1', 'Stock Price 2')
end


\end{lstlisting}

\begin{lstlisting}[frame=none]
clear 
% Define end of time interval
T=2;
N = 365;
dt = T/N;
m=1;

%Define arrays for simulation of process
W = zeros(m,N);
dW = zeros(m,N);
x= zeros(m,N); 
f= zeros(m,N);

W0 = 75;
a = @(z) 0;
sigma = 0.3;
i=1;
dW(:,1) = W0 .*( a(i*dt) .* dt + sigma .* sqrt(dt) .* randn(m,1));
W(:,1) = W0 + dW(:,1);
for i=2:N
    dW(:,i) = W(:,i-1) .*( a(i*dt).* dt+  sigma .*  sqrt(dt).*randn(m,1));
    W(:,i) = W(:,i-1) + dW(:,i);     
end

Gamma = @(t)1; %@(z) (T-z).^0.5;
r = 0.03;
c = 0.5;
A = r;
K = 30;
Q= @(x) exp(2*A*(T-x)).*Gamma(x).^(-1); 
R = @(s) quad(Q,s,T); 
M=0;
d1 = @(q) (log(W(q)/K) + (T-q*dt)*(r+sigma.^2/2))/(sigma*sqrt(T-q*dt));
d2 = @(q) d1(q) - sigma*sqrt(T-q*dt);

d10 = (log(W0/K) + (T)*(r+sigma.^2/2))/(sigma*sqrt(T)) ;
d20 = d10 - sigma*sqrt(T);
H0 = normcdf(d10)*W0 - normcdf(d20)*K*exp(-r*T);


for q = 1:N
    df = normcdf(d1(q))*sigma*dW(:,q);
    if q == 1
        f(:,q) = max(H0 + df,0);
    else
        f(:,q) = max(f(:,q-1) + df,0);
    end
    
    t = q*dt;
    M = M + R(t).^(-1)* df;
    mu = R(0).^(-1)*(H0 ) + M;
    u = c*Gamma(t).^(-1)*exp(A*(T-t))*mu;
    if q==1
        x(:,q) = exp(r*dt).*(u*dt);
    else 
        x(:,q) = (x(:,q-1) + u*dt).*exp(r*dt);
    end

end   

figure
plot(0:dt:T, c*[H0,f]);
hold on
plot(0:dt:T, [0,x]);
xlabel('Time (years)')
ylabel('Value ($)')
legend( 'Equity Excess', 'Accumulated Cash')

\end{lstlisting}
